# Supplementary material for: Sparse and Low-Rank High-Order Tensor Regression via Parallel Proximal Method
Source: arXiv:1911.12965 source file (2023-08-09)
Supplement: Supplementary file 1 [file appendix.tex]

\section{More on Background}
    \subsection{Tensor and Related Operations}
    
        \begin{definition}
            \textbf{($\mathbf{M}$-order tensor)} Tensor data, also known as multidimensional array, is a general data form with multiple dimensionalities. Specifically, a $M$-order tensor $\mathcal{A} \in \mathbb{R}^{p_1 \times p_2 \times \cdots \times p_M}$ has $M$ dimensions (or $M$ orders) in total. Specifically, a 1-mode tensor is a vector and a 2-order tensor is a matrix.
        \end{definition}
    
        \begin{definition}
            \textbf{(Vectorizing and tensorizing)} Vectorizing, denoted as $\mathcal{V}(\cdot)$, is the process of stacking elements of a $M$-order tensor into a vector with the corresponding size $\mathbb{R}^{p_1 * \cdots * p_M}$. Tensorizing, denoted as $\mathcal{T}_\mathcal{P}(\cdot)$, is the reverse process of vectorizing, which rearranges a vector into a tensor based on the size of each mode $\mathcal{P}=\{p_1,\cdots,p_M\}$. Notably, the order of traversing elements for both vectorizing and tensorizing should be the same. Take a $2 \times 3$ tensor as an example. Assume we have 
            \begin{equation}
                \mathcal{A} = \left[
                \begin{aligned}
                    &1 \qquad 2 \qquad 3 \\
                    &4 \qquad 5 \qquad 6
                \end{aligned}
                \right] \in \mathbb{R}^{2 \times 3}.
            \end{equation}
            Then vectorizing it by traversing the first dimension firstly and traversing the second dimension in the next, we have
            \begin{equation}
                \mathbf{a} = \mathcal{V}(\mathcal{A}) = [1 \qquad 4 \qquad 2 \qquad 5 \qquad 3 \qquad 6] \in \mathbb{R}^6.
            \end{equation}
        Further tensorizing it with $\mathcal{T}_{\mathcal{P}}(\mathbf{a})$ given $\mathcal{P}=\{2, 3\}$ needs to put $1$ at location $(1,1)$, put $4$ at location $(2,1)$, and locate other elements respectively in the same way. Therefore, in this way, the tensorizing and vectorizing are a pair of inverse operations, and we have  $\mathcal{T}_{\mathcal{P}}(\mathcal{V}(\mathcal{A})) = \mathcal{A}$.    
        \end{definition}
        
        \begin{definition}
            \textbf{(Tensor unfolding and folding)} Unfolding, also known as matricization, is the procedure of rearranging a tensor into a matrix. The result of tensor unfolding is determined by the mode along which the tensor is unfolded. For example, a $3 \times 4 \times 5$ tensor can be unfolded into a $3 \times 20$ matrix along the first order or a $12 \times 5$ matrix along the second order, and so on. Unfolding a tensor along the $m$-order is denoted by $\mathcal{U}_m(\mathcal{A}) = A_{(m)}$, which collect the fibers of mode $n$ to be columns of the resulting matrix. Using notations of \cite{kolda2009tensor}, the element at location $(i_1, i_2, \cdots, i_M)$ is mapped to the matrix element at location $(i_m, j)$ where
            \begin{equation}
                j = 1 + \sum\limits_{k = 1,k \neq m}^M (i_k - 1)J_k ~~ \text{with} ~~ J_k = \prod\limits_{l=1, l \neq m}^{m-1}p_l.
            \end{equation}
            Assume w have a tensor $\mathcal{A} \in \mathbb{R}^{2 \times 2 \times 2}$ with slices of the last dimension as 
            \begin{equation}
                \mathcal{A}_{::1} = \left[
                    \begin{aligned}
                    & 1 \qquad 2 \\
                    & 3 \qquad 4
                    \end{aligned}
                \right],~~~
                \mathcal{A}_{::2} = \left[
                    \begin{aligned}
                    & 5 \qquad 6 \\
                    & 7 \qquad 8
                    \end{aligned}
                \right].
            \end{equation}
            Then unfolding $\mathcal{A}$ along every mode obtains 
            \begin{equation}
                A_{(1)} = \left[
                    \begin{aligned}
                        & 1 \qquad 2 \qquad 5 \qquad 6 \\
                        & 3 \qquad 4 \qquad 7 \qquad 8
                    \end{aligned}
                \right],
            \end{equation}
            
            \begin{equation}
                A_{(2)} = \left[
                    \begin{aligned}
                        & 1 \qquad 3 \qquad 5 \qquad 7 \\
                        & 2 \qquad 4 \qquad 6 \qquad 8
                    \end{aligned}
                \right],
            \end{equation}
            
            and 
            \begin{equation}
                A_{(3)} = \left[
                    \begin{aligned}
                        & 1 \qquad 3 \qquad 2 \qquad 4 \\
                        & 5 \qquad 7 \qquad 6 \qquad 8
                    \end{aligned}
                \right],
            \end{equation}
        Notice that different papers might use different orderings of the columns for mode $m$ unfolding. However, in general and specifically in this paper, the ordering of columns is not important. 
        
        Similar to tensorizing and vectorizing, folding operation is the inverse operation of unfolding. Let $\mathcal{F}_m(\cdot)$ denote folding a unfolded tensor along the $m$-th mode. We have $\mathcal{F}_1(A_{(1)}) = \mathcal{A}$ and so on. Generally, $\mathcal{F}_1(\mathcal{U}_m(\mathcal{A})) = \mathcal{A}$.
        \end{definition}
        
        \begin{definition}
            \textbf{(Tensor inner product)} The inner product of two tensors $\mathcal{A}, \mathcal{B} \in \mathbb{R}|^{p_1 \times \cdots \times p_M}$ with the same size is the summation of products of all the elements.
            \begin{equation}
                <\mathcal{A}, \mathcal{B}> = \sum\limits_{i_1=1}^{p_1}\cdots\sum\limits_{i_M=1}^{p_M} \mathcal{A}_{i_1 \cdots i_M}\mathcal{B}_{i_1 \cdots i_M}
            \end{equation}
            Therefore, we have $<\mathcal{A}, \mathcal{A}> = ||\mathcal{A}||_F^2$.
        \end{definition}
        
        \begin{definition}
            \textbf{($\mathbf{m}$-mode product)} The $m$-mode product of a tensor $\mathcal{A} \in \mathbb{R}^{p_1 \times \cdots \times p_M}$ with a matrix $\mathbf{Z} \in \mathbb{R}^{J \times p_m}$ is denoted as $\mathcal{A} \times_m \mathbf{Z}$. The result is of size $p_1 \times \cdots \times p_{m-1} \times J \times p_{m+1} \times \cdots \times p_M$. Specifically, elements of the $m$-mode product are 
            \begin{equation}
                (\mathcal{A} \times_m \mathbf{Z})_{i_1 \cdots i_{m-1} j i_{m+1} \cdots i_M} = \sum\limits_{i_m = 1}^{p_m} \mathcal{A}_{i_1 \cdots i_M} \mathbf{Z}_{j i_m} 
            \end{equation}
        \end{definition}

        \begin{definition}
            \textbf{(CANDECOMP/PARAFAC decomposition)} A tensor can be factorized as a sum of outer products of component vectors. For instance, a 3-order tensor $\mathcal{A}^{J \times K \times L}$ can be factorized as
            \begin{equation}
                \mathcal{A} = \sum\limits_{r=1}^R \mathbf{a}_r \circ \mathbf{b}_r \circ \mathbf{c}_r 
            \end{equation}
            in which $R$ is a positive integer and is named CP-rank. Besides $\mathbf{a}_r \in \mathbb{R}^J$, $\mathbf{b}_r \in \mathbb{R}^K$, and $\mathbf{c}_r \in \mathbb{R}^L$ represent component vectors for each mode respectively. Specifically, each element can be written as 
            \begin{equation}
                \mathcal{A}_{jkl} = \sum\limits_{r=1}^R \mathbf{a}_{rj} \mathbf{b}_{rk} \mathbf{c}_{rl}.
            \end{equation}
        \end{definition}
        
        \begin{definition}
            \textbf{(Tucker decomposition)} The Tucker decomposition is the direct extension of singular value decomposition (SVD) to high-order data. Therefore, it is always called higher-order singular value decomposition (HOSVD) in many papers. Through Tucker decomposition, a tensor is  decomposed into a core tensor multiplied by matrices along each mode. Specifically, for the 3-order tensor $\mathcal{A} \in \mathbb{R}^{J \times K \times L}$, we have
            \begin{equation}
                \mathcal{A} = \mathcal{C} \times_1 \mathbf{X} \times_2 \mathbf{Y} \times_3 \mathbf{Z}
            \end{equation}
            in which $\mathcal{C} \in \mathbb{R}^{D \times E \times F}$ is the core tensor and $\mathbf{A} \in \mathbb{R}^{J \times D}$, $\mathbf{B} \in \mathbb{R}^{K \times E}$, $\mathbf{C} \in \mathbb{R}^{L \times F}$ are factor matrices. Elements in the core tensor $\mathcal{C}$ denotes the interaction between different components.
        \end{definition}

\section{Proximal Operators for \NAME{}}
    When solving \NAME{} with our algorithm, we need to define proximal operators for a total of four functions. Specifically, for those two functions that are relevant to $\ell_1$ norm, we have  
    
   \begin{equation}
    \text{prox}_{4\lambda||W||_1}(W) = S_{4\lambda}(W)
   \end{equation}
    and
    \begin{equation}
    \text{prox}_{||W-Z||_\infty \leq \lambda}(W) = 
    \left\{
      \begin{aligned}
        Z_{ij},&~~~~|W_{ij}-Z_{ij}| \leq \lambda \\
        Z_{ij} + \lambda,&~~~W_{ij} - Z_{ij} > \lambda \\
        Z_{ij} - \lambda,&~~~W_{ij} - Z_{ij} < -\lambda 
      \end{aligned}
    \right.
  \end{equation}
    Here, $S_\lambda(\cdot)$ is an element-wise soft-thresholding operator with $[S_\lambda(A)]_{ij} = \sign(A_{ij})\max\{|A_{ij}|-\lambda,~0\}$.

   Then, the other two nuclear-norm-relevant proximal operators are computed based on singular value decomposition (SVD). For a matrix $A$, SVD decomposes it into $A=U \Sigma V^T$ in which $\Sigma$ is a diagonal matrix with singular values on its diagonal and $U$, $V$ are left and right singular vectors correspondingly. Based on SVD, we have
   
   \begin{equation}
    \text{prox}_{4\tau||W||_*}(W) = US_{4\tau}(\Sigma)V^T
  \end{equation}
  and
  \begin{equation}
    \text{prox}_{||W-Z||_{\text{spec}} \leq \tau}(W) = 
    \left\{
      \begin{aligned}
        Z,&~~~~\sigma_{\text{max}}(\Sigma) \leq \tau \\
        US_{\tau}(\Sigma)V^T+Z,&~~~\sigma_{\text{max}}(\Sigma) > \tau 
      \end{aligned}
    \right.
  \end{equation}
%   The thresholding operator $D_\tau(\cdot)$ enforces the maximal diagonal elements of $\Sigma$ to be no more than $\tau$. Therefore, we define $[D_\tau(\Sigma)]_{ii} = \min\{\Sigma_{ii},~\tau \}$. 
    
\section{Dual Norm of the Hybrid Norm}
\begin{theorem}\label{appendix-theorem:dual-norm}
    Suppose we have the the hybrid regularizer $\mathcal{R}(w)=\sum\limits_{\beta \in I} \mathbf{c}_\beta\mathcal{R}_\beta(w_\beta)$ where $\sum\limits_{\beta \in I}w_\beta = w$ and $\mathbf{c}$ is a vector containing regularization parameter for each component norm $\mathcal{R}_\beta (\cdot)$. Then its dual norm is $\mathcal{R}^*(w) = \max\limits_{\beta \in I} \mathcal{R}_\beta^*(w_\beta)/\mathbf{c}_\beta$.
\end{theorem}

\begin{proof}
    The dual norm can be derived by
    \begin{equation}
        \begin{aligned}
        \mathcal{R}^*(w) &=\sup\limits_{u} \frac{<w, u>}{u} \\
        &= \sup\limits_{u_\beta} \frac{\sum\limits_{\beta}<w_\beta, u>}{ \sum\limits_{\beta}\mathbf{c}_\beta\mathcal{R}_\beta (w_\beta)} \\
        &= \sup\limits_{u_\beta} \frac{\sum\limits_{\beta}<w_\beta, u / \mathbf{c}_\beta>}{\sum\limits_{\beta}\mathcal{R}_\beta (w_\beta)} \\
        &\leq \sup\limits_{u_\beta} \frac{\sum\limits_{\beta} \mathcal{R}^*_\beta(u/\mathbf{c}_\beta)\mathcal{R}(w_\beta)}{\sum\limits_{\beta}\mathcal{R}_\beta (w_\beta)} \\
        &\leq \max\limits_{\beta \in I} \mathcal{R}^*_\beta(u) / \mathbf{c}_\beta.
        \end{aligned}
    \end{equation}
\end{proof}
% \vspace{-15pt}

Therefore when substituting $w$ with $\mathcal{W}=\sum_{m=1}^M \frac{1}{M}W_{(m)}$, defining $\mathbf{c}=(\lambda_1,\cdots,\lambda_M,\tau_1,\cdots,\tau_M)$ \footnote{Notice although here we let controlling parameter pairs $(\lambda_m,\tau_m)$ varies among different $m$, in our analysis of main text we let $\lambda_1 = \cdots = \lambda_M$ and $\tau_1 = \cdots = \tau_M$ for simplicity.}, and defining 
\begin{equation}
    \begin{aligned}
    \mathcal{L}(\mathcal{W})&=||y-<\mathcal{W},\mathcal{X}>||_2^2, \\
    \mathbf{c}\mathcal{R}(\mathcal{W})&=\inf\left\{\sum_{m=1}^M\mathbf{c}_m||W_{(m)}||_1 ~+ \right.\\ 
    & \qquad \left. \sum_{q=M+1}^{2M}\mathbf{c}_{q}||W_{(q-M)}||_*\right\}.
    \end{aligned}
\end{equation}
we have 
\begin{equation}
\begin{aligned}
    \mathcal{R}^*(\mathcal{W}) &=~ \max \left\{||W_{(1)}||_\infty,\cdots,||W_{(M)}||_\infty, \right. \\
    &\qquad\qquad~ \left. ||W_{(1)}||_2,\cdots,||W_{(M)}||_2 \right\}
\end{aligned}
\end{equation}

\section{Decomposability of Tensor Nuclear Norm}
\begin{theorem}\label{theorem:decomposibility}
    The tensor nuclear norm $||\mathcal{W}||_* = \frac{1}{M} \sum_{m=1}^M ||W_{(m)}||_*$ is decomposable given a pair of subspaces $(\mathcal{M}, \bar{\mathcal{M}}^\bot)$. Specifically, 
    \begin{equation}
        ||\mathcal{W} + \mathcal{V}||_* = ||\mathcal{W}||_* + ||\mathcal{V}||_*
    \end{equation}
    for all $\mathcal{W} \in \mathcal{M}(U,V)$ and $\mathcal{V} \in \bar{\mathcal{M}}^\bot(U,V)$ with $\mathcal{M}(U,V) =  \{ \mathcal{W} \in \mathbb{R}^{p_1 \times \cdots \times p_M}~|~\text{col}(W_{(1)} \subseteq U_1, \cdots, \text{col}(W_{(M)}) \subseteq U_M,~\text{row}(W_{(1)}) \subseteq V_1, \cdots,\text{row}(W_{(M)}) \subseteq V_M \}$ and $\bar{\mathcal{M}}^\bot(U,V) =  \{ \mathcal{W} \in \mathbb{R}^{p_1 \times \cdots \times p_M}~|~\text{col}(W_{(1)} \subseteq U_1^\bot, \cdots, \text{col}(W_{(M)}) \subseteq U_M^\bot,~\text{row}(W_{(1)}) \subseteq V_1^\bot, \cdots,\text{row}(W_{(M)}) \subseteq V_M^\bot \}$. Here, $\text{row}(\cdot)$ and $\text{col}(\cdot)$ are row and column space respectively. $U_m$ and $V_m$ is a pair of subspaces that $U_m \subseteq \mathbb{R}^p_m$ and $V_m \subseteq \mathbb{R}^{p_1 * \cdots * p_{m-1} * p_{m+1} * \cdots * p_M}$ for the $m$-mode unfolded tensor $W_{(m)}$.
\end{theorem}

\begin{proof}
    For an arbitrary pair of tensors $\mathcal{W} \in \mathcal{M}(U,V)$ and $\mathcal{V} \in \bar{\mathcal{M}}^\bot (U,V)$,  their $m$-mode unfolded tensor $W_{(m)}$ and $V_{(m)}$ have orthogonal row and column spaces. Because $\text{row}(W_{(m)}) \subseteq V_m$, $\text{row}(V_{(m)}) \subseteq V_m^\bot$, $\text{col}(W_{(m)}) \subseteq U_m$, $\text{col}(V_{(m)}) \subseteq U_m^\bot$, and $V_m \bot V_m^\bot$ and $U_m \bot U_m^\bot$. This implies that they satisfies the decomposability of matrix nuclear norm, namely, with a little abuse of notations, the matrix nuclear norm $||W_{(m)}+V_{(m)}||_* = ||W_{(m)}||_*+||V_{(m)}||_*$. Thus, the orthogonality of unfolded tensors are obtained. 
    
    Then, notice the unfolding operation do not change the elements of a tensor, hence, we have $(\mathcal{W}+\mathcal{V})_{(m)} = W_{(m)}+V_{(m)}$. Therefore, the tensor nuclear norm of the sum of two tensors can be reformulated as 
    \begin{equation}
        \begin{aligned}
            ||\mathcal{W}+\mathcal{V}||_* &=~\frac{1}{M}\sum\limits_{m=1}^M ||(\mathcal{W}+\mathcal{V})_{(m)}||_* \\
            &=~\frac{1}{M}\sum\limits_{m=1}^M ||W_{(m)}+V_{(m)}||_* \\
            &=~\frac{1}{M}\sum\limits_{m=1}^M \left(||W_{(m)}||_*+||V_{(m)}||_*\right) \\
            &=~||\mathcal{W}||_* + ||\mathcal{V}||_*.
        \end{aligned}
    \end{equation}
    So with the subspace pair properly defined in Theorem \ref{theorem:decomposibility}, the decomposabiltiy of tensor nuclear norm is proved.
\end{proof}

\section{Proof of Error Bound}

\textbf{(C1:sparse)} The true coefficient $\mathcal{W}^*$ is exactly sparse with $k$ non-zero elements. 

\noindent\textbf{(C2:low-rank)} The true coefficient $\mathcal{W}^*$ is a $R$-rank tensor where $R = \max\limits_{\mathcal{A} \in \mathbb{R}^{p_1 \times \cdots \times p_M}}(r_{\perp}(\mathcal{A}))$ and $r_{\perp}(\mathcal{A})$ denotes the orthogonal rank of $\mathcal{A}$. The orthogonal rank is the smallest number that satisfies $\mathcal{A}=\sum_{r=1}^{r_{\perp}(\mathcal{A})}\mathcal{U}_r$ with $<\mathcal{U}_{r_1}, \mathcal{U}_{r_2}>=0,~r_1 \neq r_2$ for $1 \leq r_1 \leq r_{\perp}(\mathcal{A}),~1 \leq r_2 \leq r_{\perp}(\mathcal{A})$. 

\vskip 10pt
\begin{theorem}\label{theorem:error-bound}
    Suppose that the true coefficient tensor $\mathcal{W}^*$ satisfies conditions \textbf{(C1:sparse)} and \textbf{(C2:low-rank)}. Furthermore, suppose we solve \NAME{} with controlling parameters $\lambda$ and $\tau$ satisfying the constraints. Then, the optimal solution satisfies the following error bound:
    \begin{equation}
        ||\widehat{\mathcal{W}}-\mathcal{W}^*||_F \leq 4\sqrt{2}\left(\lambda\sqrt{\prod\limits_{m=1}^{M}p_m}+\tau\sqrt{R}\right).
    \end{equation}
\end{theorem}

\begin{proof}
    In our method, we utilize two regularizers, element-wise $\ell_1$ norm $\mathcal{R}_1(\cdot)=||\cdot||_1$ and tensor nuclear norm $\mathcal{R}_1(\cdot)=||\cdot||_*$. Thus, firstly, let $\Delta_{1} \defeq \widehat{\mathcal{W}}_{||\cdot||_1} - \mathcal{W}^*$ and $\Delta_{2} \defeq \widehat{\mathcal{W}}_{||\cdot||_*} - \mathcal{W}^*$, where $\widehat{\mathcal{W}}_{||\cdot||_1}$, $\widehat{\mathcal{W}}_{||\cdot||_*}$ are solutions of minimizing element-wise $\ell_1$ norm and tensor nuclear norm correspondingly. Moreover, let $\Delta \defeq \Delta_{1}+\Delta_{2}$, tuning parameter $\beta = \lambda$, $\beta_2 = \tau$, and $\mathcal{I}=\{1,2\}$. Then, the Frobenius error $||\Delta||_F$ is bounded as following:
    \begin{equation}\label{eq:proof-1}
        \begin{aligned}
        ||\Delta||^2_F &=  < \Delta,\Delta > = \sum\limits_{\alpha \in \mathcal{I}} < \Delta, \Delta_\alpha > \\
        &\leq \sum\limits_{\alpha \in \mathcal{I}}|< \Delta, \Delta_\alpha >| \\
        &\leq 2\sum\limits_{\alpha \in \mathcal{I}} \beta_\alpha\mathcal{R}_{\alpha}(\Delta_\alpha)\\
        &\leq 2\sum\limits_{\alpha \in \mathcal{I}} \beta_\alpha\left\{\mathcal{R}_{\alpha}[\Pi_{\Bar{\mathcal{M}}_\alpha}(\Delta_\alpha)]+\beta_\alpha\mathcal{R}_{\alpha}[\Pi_{\Bar{\mathcal{M}}_\alpha^\perp}(\Delta_\alpha)]\right\}\\
        &\leq 4\sum\limits_{\alpha \in \mathcal{I}}\beta_\alpha\mathcal{R}_{\alpha}[\Pi_{\Bar{\mathcal{M}}_\alpha}(\Delta_\alpha)]\\
        %&\leq 4\sum\limits_{\alpha \in \mathcal{I}}\beta_\alpha\Psi(\Bar{\mathcal{M}}_\alpha)||\Pi_{\Bar{\mathcal{M}}_\alpha}(\Delta_\alpha)||_F.
        \end{aligned}
    \end{equation}

    Here, the second inequality comes from an application of H\"older's inequality that for each $\alpha \in \mathcal{I}$, $|\ll \Delta,\Delta_\alpha \gg| \leq \mathcal{R}_\alpha^*(\Delta)\mathcal{R}_\alpha(\Delta_\alpha) \leq 2\beta_\alpha\mathcal{R}_\alpha(\Delta_\alpha)$, where $\ll A,B \gg=\sum_i\sum_jA_{ij}B_{ij}$ denotes the trace inner product. At here, we let $\Psi(\Bar{\mathcal{M}}_\alpha)$ demonstrate the compatibility of space $\Bar{\mathcal{M}}_\alpha$ as following:
    \begin{equation}\label{eq:space-compatibility}
        \Psi(\Bar{\mathcal{M}}_\alpha) \defeq \sup\limits_{U \in \Bar{\mathcal{M}}_\alpha \backslash \mathbf{0}}\frac{\mathcal{R}_\alpha(U)}{||U||_F}.
    \end{equation}
    With this, \eref{eq:proof-1} can be rewritten as 
    \begin{equation}\label{eq:proof-2}
        ||\Delta||_F^2 \leq 4\sum\limits_{\alpha \in \mathcal{I}}\beta_\alpha\Psi(\Bar{\mathcal{M}}_\alpha)||\Pi_{\Bar{\mathcal{M}}_\alpha}(\Delta_\alpha)||_F.
    \end{equation}
    Now, we consider about the term $||\Pi_{\Bar{\mathcal{M}}_\alpha}(\Delta_\alpha)||_F$. Notice that the projection operator is defined in terms of the Frobenius norm, which makes it non-expensive for all $\alpha$ such that $||\Pi_{\Bar{\mathcal{M}}_\alpha}(\Delta_\alpha)||_F \leq ||\Delta_\alpha||_F$. Moreover, similar to \eref{eq:proof-1} and \eref{eq:proof-2}, we have $||\Delta_\alpha||_F^2 \leq 4\beta_\alpha\Psi(\Bar{\mathcal{M}}_\alpha)||\Pi_{\Bar{\mathcal{M}}_\alpha}(\Delta_\alpha)||_F$.
    %\notice{compared to SEE, two conditions less are needed} 
    Hence, we obtain
    \begin{equation}\label{eq:proof-3}
        \begin{aligned}
        (\sum\limits_{\alpha \in \mathcal{I}}||\Pi_{\Bar{\mathcal{M}}_\alpha}(\Delta_\alpha)||_F)^2 &\leq (\sum\limits_{\alpha \in \mathcal{I}}||\Delta_\alpha||_F)^2\\
        & \leq |\mathcal{I}|\sum\limits_{\alpha \in \mathcal{I}}||\Delta_\alpha||^2_F\\
        & \leq 4|\mathcal{I}|\beta_\alpha\Psi(\Bar{\mathcal{M}}_\alpha)||\Pi_{\Bar{\mathcal{M}}_\alpha}(\Delta_\alpha)||_F,
        \end{aligned}
    \end{equation}
    therefore, 
    \begin{equation}\label{eq:proof-4}
        \sum\limits_{\alpha \in \mathcal{I}}||\Pi_{\Bar{\mathcal{M}}_\alpha}(\Delta_\alpha)||_F \leq 4|\mathcal{I}|\beta_\alpha\Psi(\Bar{\mathcal{M}}_\alpha).
    \end{equation}
    Plugging \eref{eq:proof-4} back into \eref{eq:proof-2}, the Frobenius norm error bound is derived as 
    \begin{equation}\label{eq:proof-5}
        ||\Delta||_F^2 \leq 16|\mathcal{I}|(\sum\limits_{\alpha \in \mathcal{I}}\beta_\alpha \Psi(\Bar{\mathcal{M}}_\alpha))^2,
    \end{equation}
    hence,
    \begin{equation}\label{eq:proof-6}
        ||\Delta||_F \leq 4\sqrt{|\mathcal{I}|}\sum\limits_{\alpha \in \mathcal{I}}\beta_\alpha \Psi(\Bar{\mathcal{M}}_\alpha).
    \end{equation}
    Revisit the formulation of our method, we have $\mathcal{I}=\{1,2\}$ and $\mathcal{R}_1(\Delta_1)=||\Delta_1||_1$, $\mathcal{R}_2(\Delta_2)=||\Delta_2||_*$. For $\ell_1$ norm $\mathcal{R}_1(\Delta_1) = ||\Delta_1||_1$, \cite{negahban2012unified} has already proved its decomposability. Hence, it can easily obtained that 
    \begin{equation}\label{eq:compatilibility-l1}
        \Psi(\Bar{\mathcal{M}}_1) = \sup\limits_{\mathcal{U} \in \Bar{\mathcal{M}}_\alpha \backslash \mathbf{0}}\frac{||\mathcal{U}||_1}{||\mathcal{U}||_F} \leq \sqrt{\prod\limits_{m=1}^{M}p_m}.
    \end{equation}
    As for the tensor nuclear norm $\mathcal{R}_2(\Delta_2)=||\Delta_2||_*$, we already proved its decomposability in this paper and a few previous works \cite{friedland2018nuclear,kong2018new} have proven its upper bound. To our best knowledge, \cite{kong2018new} propose the most tightest upper bound of tensor nuclear norm given by the Frobenius norm, which is $||\mathcal{A}||_* \leq \sqrt{R}||\mathcal{A}||_F$. Here, $R = \max\limits_{\mathcal{B} \in \mathbb{R}^{p_1 \times p_M}} \{\text{rank}_{\perp}\mathcal{B}\}$, in which $\text{rank}_{\perp}(\mathcal{B})$ denotes the orthogonal rank of an arbitrary nonzero tensor $\mathcal{B}$. Therefore, we have
    \begin{equation}\label{eq:compatibility-2}
        \Psi(\Bar{\mathcal{M}}_2) = \sup\limits_{\mathcal{U} \in \Bar{\mathcal{M}}_\alpha \backslash \mathbf{0}}\frac{||\mathcal{U}||_*}{||\mathcal{U}||_F} \leq \sqrt{R}.
    \end{equation}
    Integrating $\Psi(\Bar{\mathcal{M}}_1)$, $\Psi(\Bar{\mathcal{M}}_2)$ with \eref{eq:proof-6}, we finally have the following error upper bound:
    \begin{equation}\label{eq:final-bound-1}
        ||\Delta||_F \leq 4\sqrt{2}\left(\lambda\sqrt{\prod\limits_{m=1}^{M}p_m}+\tau\sqrt{R}\right).
    \end{equation}
\end{proof}

\begin{corollary}\label{corollary:error-bound-3D}
    If the coefficient is a 3-order tensor such that $\mathcal{W} \in \mathbb{R}^{p_1 \times p_2 \times p_3}$ and condition \textbf{(C1:sparse)} and \textbf{(C2:low-rank)}  hold, the optimal solution of \NAME{} satisfies the following error bound:
    \begin{equation}
        ||\widehat{\mathcal{W}}-\mathcal{W}^*||_F \leq 4\sqrt{2}\left(\lambda\sqrt{\prod\limits_{m=1}^{M}p_m}+\tau R^\prime\right)
    \end{equation}
    where 
    \begin{equation}
        \begin{aligned}
            R^\prime = \max&\left\{\sqrt{r_1\min\{r_2,r_3\}},\sqrt{r_2\min\{r_1,r_3\}}, \right. \\
            &\quad \left. \sqrt{r_3\min\{r_1,r_2\}}\right\}
        \end{aligned} 
    \end{equation}
    and $r_m = \text{rank}(W_{(m)})$ denotes the rank of the unfolded tensor.
\end{corollary}

\begin{proof}
    Specifically for 3-order tensor, \cite{kong2018new} propose the upper bound of tensor nuclear norm given by nuclear norms of its unfolding matrices. Specifically, let $r_m = \text{rank}(W_{(m)}),~m=1,2,3$, then
    \begin{equation}\label{eq:unfolding-nuclear-norm-bound}
        \begin{aligned}
            ||\Delta||_* \leq & \frac{1}{3}\left(\sqrt{\min\{r_2,r_3\}}||\Delta_{(1)}||_* \right.\\ 
            &\qquad + \left. \sqrt{\min\{r_1,r_3\}}||\Delta_{(3)}||_*\right. \\
            &\qquad +\left. \sqrt{\min\{r_1,r_2\}}||\Delta_{(3)}||_*\right)\\
            \leq & \frac{1}{3}\left(\sqrt{r_1\min\{r_2,r_3\}}||\Delta||_F \right. \\
            &\qquad \left. +\sqrt{r_2\min\{r_1,r_3\}}||\Delta||_F \right. \\
            &\qquad +\left. \sqrt{r_3\min\{r_1,r_2\}}||\Delta||_F\right)\\
            \leq & \max\{\sqrt{r_1\min\{r_2,r_3\}},\sqrt{r_2\min\{r_1,r_3\}},\\
            &\qquad \sqrt{r_3\min\{r_1,r_2\}}\}||\Delta||_F.
        \end{aligned}
    \end{equation}
    Therefore, $\Psi(\Bar{\mathcal{M}}_2)$ becomes
    \begin{equation}\label{eq:compatibility-3}
       \begin{aligned}
        \Psi(\Bar{\mathcal{M}}_2) &= \sup\limits_{\mathcal{U} \in \Bar{\mathcal{M}}_\alpha \backslash \mathbf{0}}\frac{||\mathcal{U}||_*}{||\mathcal{U}||_F} \\
        &\leq \max\{\sqrt{r_1\min\{r_2,r_3\}},\sqrt{r_2\min\{r_1,r_3\}}, \\
        & \qquad\qquad \sqrt{r_3\min\{r_1,r_2\}}\}. 
       \end{aligned}
    \end{equation}
    Substituting $\Psi(\Bar{\mathcal{M}}_2)$ with \eref{eq:compatibility-3} in \eref{eq:proof-6}, we have the final error bound
    \begin{equation}\label{eq:final-bound-2}
        \begin{aligned}
            ||\Delta||_F &\leq 4\sqrt{2}(\lambda\sqrt{\prod\limits_{m=1}^{M}p_m}+\tau\max\{\sqrt{r_1\min\{r_2,r_3\}},\\
            & \mspace{80mu} \sqrt{r_2\min\{r_1,r_3\}},\sqrt{r_3\min\{r_1,r_2\}}).
        \end{aligned}
    \end{equation}
\end{proof}

\iffalse
\begin{theorem}
    For each subproblem \eref{eq:subproblem}, every sequence $(W_m^t)_{1 \leq t \leq \text{iter}}$ generated by Algorithm \ref{algo:pseudo} converges to a solution to \eref{eq:subproblem}. 
\end{theorem}

\begin{proof}
    \cite{combettes2011proximal} propose the parallel proximal method for minimizing the summation of several functions, such that 
    \begin{equation}\label{eq:summation-functions}
        \begin{aligned}
        \min\limits_{x_1,x_2,\cdots,x_D}&~f_1(x_1)+f_2(x_2)+\cdots+f_D(x_D) \\
        \text{s.t.}&~~~x_1 = x_2 = \cdots = x_D.
        \end{aligned}
    \end{equation}
    Notice that our \eref{eq:proximal-problem} coincides with the structure of \eref{eq:summation-functions} with $D=4$. Therefore, due to the \textbf{Proposition 7.3}, our subproblem also converges. 
\end{proof}
\fi

\section{More Related Works Involving Tensor}

Some other models were proposed for other problem settings. Recently, \cite{hao2019sparse,imaizumi2016doubly,yu2017tensor,guhaniyogi2017bayesian} propose models for non-parametric estimation by assuming that the response $y = f(\mathcal{X}) + \varepsilon$, making use of either additive model or Bayesian approaches (e.g., Gaussian process). Apart from the above-mentioned ones, many models \cite{sun2017store,raskutti2019convex,yu2016learning,zhu2009intrinsic,li2011multiscale} were put forward to estimate the relationship between the variable tensor $\mathcal{X}$ and a response tensor $\mathcal{Y}$. Because these methods have different objectives from our method, we pay little attention to them and exclude them from experiments. 

 Another line of statistical models involving tensor data is tensor decomposition \cite{kolda2009tensor,sun2017provable,allen2012sparse,li2017model,madrid2017tensor}. Tensor decomposition can be considered an unsupervised problem that aims at approximating the tensor with lower-order data. On the contrary, our \NAME{}{} is a supervised method estimating the latent relationship between variables and responses. Because these methods have different objectives from our method, we pay little attention to them and exclude them from experiments.

\section{More on Experiment}
\subsection{Experiment Setups}

\paragraph{Datasets:} We compare \NAME{} with baselines on simulated datasets and a real-world fMRI dataset. Specifically, our simulated datasets are generated through several steps:
\begin{enumerate}
    \item [1.] Generate $\mathcal{W} \in \mathbb{R}^{p_1 \times p_2 \times \cdots \times p_M}$ and $\mathcal{X} \in \mathbb{R}^{N \times p_1 \times p_2 \times \cdots \times p_M}$ with each element drawn from the normal distribution $\mathcal{N}(0,1)$. 

    \item [2.] Randomly set $s\%$ elements of $\mathcal{W}$ to be $0$. 

    \item [3.] Compute the response $y \in \mathbb{R}^{N}$ with respect to $y_i = <\mathcal{W},\mathcal{X}_i>+\alpha\varepsilon_i$. Here, $\alpha$ controls the ratio of noises and the noise $\varepsilon_i$ is generated from the normal distribution $\mathcal{N}(0,1)$.
\end{enumerate}
To test \NAME{} and other methods on various simulated datasets, we generate multiple simulated datasets based on settings shown in Table \ref{appendix-tab:simulated-descrip}. In addition to simulated datasets, we further experiment \NAME{} on UCF101 datasets \cite{soomro2012ucf101}.

\begin{table}[!htbp]
  \centering
  \caption {Parameter settings for data simulation. s\% denotes the sparsity level and $\alpha$ represents the noise factor.}
  \label{appendix-tab:simulated-descrip}
  %\vskip 0.1in
  \resizebox{\columnwidth}{!}{%
  \begin{tabular}{c|c|c|c|c}
  \Xhline{1.2pt}
   D1ata order &  Size (variable number) & N (sample number) & s\% (sparsity) & $\alpha$(noise)\\ 
  \cline{1-5}
%   \multirow{4}{*}{2-order data} & 15 $\times$ 15 & 112 & \multirow{16}{*}{80\%} & \multirow{16}{*}{0.1} \\
%   & 20 $\times$ 20 & 200 & & \\
%   & 25 $\times$ 25 & 312 & & \\
%   & 30 $\times$ 30 & 450 & & \\
%   \cdashline{1-3}[0.8pt/2pt]
  \multirow{7}{*}{3-order data} & 10 $\times$ 10 $\times$ 5 & 40 & \multirow{12}{*}{80\%} & \multirow{12}{*}{0.1} \\
   & 15 $\times$ 15 $\times$ 5 & 90 & & \\ 
   & 20 $\times$ 20 $\times$ 5 & 160 & & \\ 
   & 25 $\times$ 25 $\times$ 5 & 250 & & \\ 
   & 30 $\times$ 30 $\times$ 5 & 360 & & \\ 
   & 35 $\times$ 35 $\times$ 5 & 400 & & \\ 
   & 40 $\times$ 40 $\times$ 5 & 640 & & \\ 
  \cdashline{1-3}[0.8pt/2pt]
  \multirow{5}{*}{4-order data} & 10 $\times$ 10 $\times$ $\times$ 5 & 400 & & \\
   & 15 $\times$ 15 $\times$ 10 $\times$ 5 & 900 & & \\ 
   & 20 $\times$ 20 $\times$ 10 $\times$ 5 & 1600 & & \\ 
   & 25 $\times$ 25 $\times$ 10 $\times$ 5 & 2500 & & \\ 
   & 30 $\times$ 30 $\times$ 10 $\times$ 5 & 3600 & & \\ 
  \Xhline{1.2pt}
  \end{tabular}
  }
\end{table}

\paragraph{Other setups:} In the experiments, all the tuning parameters of all the methods are selected through 5-fold cross-validation procedures which take the average MSE on validation datasets as the selecting criteria. The range of tuning parameters from which we select through cross-validation is shown in Table \ref{appendix-tab:parameter-range}.  As for the experiment environment, all the experiments are implemented on a Linux server with 2 Intel Xeon Silver 4216 CPUs and 256 GB RAMs. Moreover, out of the fairness of comparison, we use MATLAB to implement all the methods. We set the maximal number of iterations to be $1000$ for all the methods and let them terminate when $\frac{||\mathcal{W}^{t+1}-\mathcal{W}^t||_F}{||\mathcal{W}^t||_F} \leq 10^{-4}$. We run every single experiment 10 times and report the average performance over these ten trials.  

\begin{table*}[!htbp]
  \centering
  \caption {Range of tuning parameters of all the methods.}
  \label{appendix-tab:parameter-range}
  %\vskip 0.1in
  \resizebox{.8\textwidth}{!}{%
  \begin{tabular}{c|c|c}
  \Xhline{1.2pt}
  Method & Parameter & CV Range \\ 
  \cline{1-3}
  \multirow{3}{*}{\NAME{}} & $\epsilon$ & $\{0, 0.1, 0.2, 0.3, 0.4, 0.5\}$\\ 
   & $\lambda$ & $\{0, 10^{-4}, 5*10^{-4}, 10^{-3}, 5*10^{-3}, 10^{-2}, 5*10^{-2}\}$\\
   & $\tau$ & $\{0, 10^{-2}, 5*10^{-2}, 10^{-1}, 5*10^{-1}, 10^0, 5*10^0, 10^1, 5*10^1\}$\\
  \cdashline{1-3}[0.8pt/2pt]
  \multirow{2}{*}{Remurs} & $\alpha$ & $\{10^-{2}, 5*10^{-2}, 10^{-1}, 5*10^{-1}, 10^0, 5*10^0, 10^1, 5*10^1\}$ \\
   & $\beta$ & $\{10^{-2}, 5*10^{-2}, 10^{-1}, 5*10^{-1}, 10^0, 5*10^0, 10^1, 5*10^1\}$ \\
   \cdashline{1-3}[0.8pt/2pt]
   Lasso & number of $\lambda$ & 100 (number of sparsity controlling parameter $\lambda$) \\
   \cdashline{1-3}[0.8pt/2pt]
   \multirow{2}{*}{Elastic Net} & number of $\lambda$ & 100 (number of sparsity controlling parameter $\lambda$) \\
    & $\alpha$ & 0.5 (trade off between $\ell_1$ and $\ell_2$ norm) \\
   \cdashline{1-3}[0.8pt/2pt]
   \multirow{3}{*}{SURF} & $\alpha$ & $\{5*10^{-4}, 10^{-4},5*10^{-3},10^{-2},5*10^{-2},10^{-1}\}$ \\
    & $\epsilon$ & $\{5*10^{-4}, 10^{-4},5*10^{-3},10^{-2},5*10^{-2},10^{-1}\}$ \\
    & R & $\{1,2,3,4,5,6,7,8,9,10\}$ \\
    \cdashline{1-3}[0.8pt/2pt]
    GLTRM & R & $\{1,2,3,4,5,6,7,8,9,10\}$ \\
  \Xhline{1.2pt}
  \end{tabular}
  }
\end{table*}

\subsection{Experiments on Simulated Data}
Table \ref{tab:MSE} shows methods' MSE values on simulated datasets. Results indicate that in most cases, \NAME{} obtains the best solution, while in other cases, an estimation computed by \NAME{} is only a little worse than the best. Therefore, \NAME{} is able to spend much less time obtaining a solution no worse than the best solutions obtained by baseline methods.

\begin{table}
  \centering
  \caption {MSE on simulated datasets with different sizes of data. The bold number denotes the best MSE value, and the underlined value represents the second-best result. Note that SURF is infeasible for 2D and 4D data, and GLTRM is only feasible for 2D data.}
  \label{tab:MSE}
  %\vskip 0.1in
  \resizebox{\columnwidth}{!}{%
  \begin{tabular}{cccccc}
  \Xhline{1.2pt}
  size & \NAME{}{} & Remurs & SURF & Lasso & Elastic Net \\ 
  \cline{1-6}
  \multicolumn{6}{c}{\emph{3D Data} -- 8\% samples}\\
  10 $\times$ 10 $\times$ 5 & \underline{0.8532} & 0.8538 & 0.8472 & 1.7993 & 1.799 \\
  15 $\times$ 15 $\times$ 5 & \underline{0.9892} & 0.9867 & 0.9994 &  2.3151 & 2.3132 \\
  20 $\times$ 20 $\times$ 5 & \underline{0.9383} & 0.9378 & 1.0049 &  2.5469 & 2.5193 \\
  25 $\times$ 25 $\times$ 5 & \textbf{0.9275} & 0.9398 & 0.9391 &  2.0149 & 2.0149 \\
  30 $\times$ 30 $\times$ 5 & \textbf{0.9186} & 0.919 & 0.9289 &  1.9381 & 1.9377 \\
  35 $\times$ 35 $\times$ 5 & \textbf{0.9336} & 0.9370 & 0.9527 &  2.0147 & 2.0147 \\
  40 $\times$ 40 $\times$ 5 & \underline{0.9073} & 0.9072 & 1.0006 & 2.1059 & 2.1065 \\
  \cdashline{1-6}[0.8pt/2pt]
  \multicolumn{6}{c}{\emph{4D Data} -- 8\% samples}\\
  10 $\times$ 10 $\times$ 10 $\times$ 5 & \textbf{0.9183} & 0.9339 & \multirow{4}{*}{\emph{N/A}} & 1.9799 & 1.9985\\
  15 $\times$ 15 $\times$ 10 $\times$ 5 & \textbf{0.9127} & 0.9186 &  & 2.1690 & 2.1690\\
  20 $\times$ 20 $\times$10 $\times$ 5 & \textbf{0.9150} & 0.9177 &  & 2.1388 & 2.1373\\
  25 $\times$ 25 $\times$10 $\times$ 5 & \textbf{0.9071} & 0.9101 &  & 1.9696 & 1.9696\\
  30 $\times$ 30 $\times$10 $\times$ 5 & \textbf{0.9110} & 0.9123 &  & 1.9754 & 1.9745\\

  \Xhline{1.2pt}
  \end{tabular}
  }
  \vspace{-10pt}
\end{table}

In addition, we test \NAME{} in high-dimensional settings. We let the shape of data be $20 \times 20 \times 5$ and vary $N$ from 50 to 400. The sparsity level is $s\%=80\%$, and the noise factor is set to $\alpha=0.1$. The MSE values shown in Table \ref{tab:high-dimensional} indicate that \NAME{} obtains the best solution under almost all conditions. Note that for $N=150$, even the MSE of \NAME{} is $0.9295$, which is a little worse than the MSE of Remurs (0.9190), it is much better than others: SURF MSE=0.9953 and Elastic Net MSE=1.6502. 

\begin{table}
  \centering
  \caption {MSE of every method in high-dimensional settings. Simulated datasets are generated with the shape of data as $20 \times 20 \times 5$, sparsity level $s\%=80\%$, and noise coefficient $\alpha = 0.1$. The number of samples varies from 50 to 400. Note that GLTRM is inapplicable for 3D data. The bold number denotes the best MSE value, and the underlined value represents the second-best result.}
  \label{tab:high-dimensional}
  %\vskip 0.1in
  \resizebox{\linewidth}{!}{%
  \begin{tabular}{ccccccccccccccc}
  \Xhline{1.2pt}
  N & \NAME{}{} & Remurs & SURF & Lasso & Elastic Net \\
  \cline{1-6}
  50 & \textbf{1.6123} & 1.6198 & 1.6439 &4.5083 & 4.5759 \\
  100 & \textbf{1.0798} & 1.0946 & 1.7101 &1.6433 & 1.6433 \\
  150 & \underline{0.9295} & 0.9190 & 0.9953 &1.6777 & 1.6502 \\
  200 & \textbf{0.8351} & 0.8469 & 0.8376 & 1.9072 & 0.8376 \\
  250 & \textbf{0.7130} & 0.7267 & 0.7199 & 1.3757 & 1.3708 \\
  300 & \textbf{0.7282} & 0.7325 & 0.7524 & 1.7316 & 1.6938 \\
  350 & \textbf{0.6275} & 0.6275 & 0.6379 & 1.3207 & 1.2804 \\ 
  400 & \textbf{0.5954} & 0.5969 & 0.5975 & 1.1487 & 1.1450 \\
  \Xhline{1.2pt}
  \end{tabular}
  }
  \vspace{-10pt}
\end{table}

In order to test the stability of \NAME{} and its sensitiveness to the sparsity level, we generate simulated datasets varying the sparsity level $s\%$ from $\{10\%, 20\%, \cdots, 90\%\}$. The shape of each sample is $20 \times 20 \times 5$, and a total of 160 samples are generated. We generate different datasets on different trials. The averaged time cost and 70\% of the variance of 10 trials are reported in \figref{fig:time-variance-sparsity}. Apparently, under every setting, \NAME{} outperforms others. Moreover, the time cost variance of \NAME{} is at most \textbf{$0.0006$}, which is much less than it of SURF and Remurs (at least $0.2$). Although LR methods also have small time variance, they might obtain a worse solution than \NAME{} (see \tabref{tab:MSE}). Therefore, \NAME{} is faster than other methods on datasets with different sparsity levels, and it is more stable. 

\begin{figure*}[!htb]
    \centering
    \includegraphics[width=2\columnwidth]{time_vs_sparsity(all).pdf}
     \caption{The time cost of \NAME{} and baselines on simulated datasets of different sparsity levels. The $70\%$ of variance of time cost is also reported for every experiment. The size of the coefficient tensor is $20 \times 20 \times 5$ and $N=160$. We let noise ratio $\alpha=0.1$.}
     \label{fig:time-variance-sparsity}
\end{figure*}

\subsection{Parameter Tuning on Action Recognition Video Dataset}
On the UCF101 dataset, we also conduct a 5-fold cross-validation to tune method hyper-parameters. In \NAME{}, we select $\tau$ from $10^{-2}$ to $1$, select $\lambda$ from $10^{-4}$ to $5\times 10^{-3}$, and select $\varepsilon$ from $0.1$ to $0.4$. In Remurs, we select both parameters ($\alpha$ and $\beta$) from $5\times10^{-3}$ to $5$. In SURF, we select $\alpha$ from $5\times10^{-4}$ to $0.1$, select $\varepsilon$ from $5\times10^{-4}$ to $0.1$, and select $R$ from $\{1, 2\}$. We randomly select 80\% of samples as training set, and the remaining are testing samples.

\newpage
\bibliography{citations}
\bibliographystyle{apalike}
